# Supplementary material for: Width-parameterized SAT: Time-Space Tradeoffs
Source: arXiv:1108.2385 source file (2011-08-11)
Supplement: Supplementary file 1 [file appendix.tex]

\subsection {Proof of Lemma \ref{lem:assignment_count}}

\begin{proof}

Denote $X^{*} = \cup_{v_i\in S}{X_i}$, since $|X^{*}|\leq
\sum_{v_i\in S}|X_i|\leq |S|\tw(\phi)$, the number of variables and
clauses in $X^{*}$ are at most $|S|\tw(\phi)$. So the number of
assignment is at most $2^{|S|\tw(\phi)}$.

\end{proof}

\subsection {Proof of Lemma \ref{lem:assignment_consistent_count}}

\begin{proof}
For a tree $\mathcal{T}$ with cutting nodes $S$, cutting a node $p$
result in several subtrees $\{\mathcal{T}_i\}$.

For each variable $x$ in node $p$, there are at most $2\leq d$
possible assignments of $x$ in subtrees $\{\mathcal{T}_i\}$.

For each clause $C$ in node $p$, if $C$ appears in $R_{\mathcal{T}}$
and is assigned $0$, according the Definition
\ref{def:assignment_consistent}, all $C$ in $\{\mathcal{T}_i\}$ are
assigned $0$, otherwise, $C$ in exactly one $\{\mathcal{T}_i\}$ is
assigned $1$, in this case, there are at most $d$ possible
assignments.

\end{proof}

\subsection {Proof of Theorem~\ref{thm:satisfiable}}

\begin{proof}

For a tree $\mathcal{T}$ with cutting nodes $S$, cutting a node $p$
result in several subtrees $\{\mathcal{T}_i\}$.

On one hand, if assignment $R_{\mathcal{T}}$ is \emph{satisfiable},
by Definition \ref{def:satisfiable}, there exists a truth assignment
on variables within $T$. Using the truth assignment, we can always
find assignments $R_{\mathcal{T}_i}$ consistent with
$R_{\mathcal{T}}$, such that the truth assignment also satisfied all
conditions in Definition \ref{def:satisfiable} on subtrees
$\mathcal{T}_i$, thus assignments $R_{\mathcal{T}_i}$ are also
\emph{satisfiable}.

On the other hand, if there exists assignments $R_{\mathcal{T}_i}$
of subtrees $\mathcal{T}_i$, such that assignments
$R_{\mathcal{T}_i}$ are consistent with $R_{\mathcal{T}}$ and all
$R_{\mathcal{T}_i}$ are \emph{satisfiable}. For each subtree
$\mathcal{T}_i$, there exists a truth assignment satisfied all
conditions in Definition \ref{def:satisfiable}. Since all these
truth assignment agree with all common variables, we can get a truth
assignment by union of them, which satisfied all conditions in
Definition \ref{def:satisfiable}. Therefore, assignment
$R_{\mathcal{T}}$ is \emph{satisfiable}.

\end{proof}

%\subsection {Proof of Theorem \ref{the:assignment_correctness}}

%\begin{proof}
%Since no previous cutting nodes in the tree decomposition
%$\mathcal{T}$, instance $\phi$ of $\sat$ is satisfiable if and only
%if the empty string $R_{\mathcal{T}}$ is satisfiable. By Lemma
%\ref{thm:satisfiable}, since tree $\mathcal{T}$ contains all
%variables, $\phi$ is satisfiable if and only if for each cut, there
%exist consistent assignments for all subtrees.
%\end{proof}

\subsection {Proof of Lemma \ref{lem:assignment_consistent_count_important}}

\begin{proof}
For a tree $\mathcal{T}$ with cutting nodes $S$, cutting a node $p$
result in several subtrees $\{\mathcal{T}_i\}$.

To proof this lemma, we want to show that, for each variable or
clause, there are at most $d$ possible combination of assignments of
it in all subtrees $\mathcal{T}_i$.

For each variable $x$, there are at most $2\leq d$ possible values.

For each clause $C$, let $d_0(d_0\leq d)$ be the number of subtrees
cut by $p$.

If $C$ does not exists in any previous cutting node, it implies that
$C$ only appears in tree $\mathcal{T}$, so there are $d_0$ possible
assignments of $C$, the $i$-th assignments set the value of $C$ in
subtree $\mathcal{T}_i$ to $1$ and rests are $0$.

If $C$ exists in some previous cutting nodes, and its value is fixed
in $\epsilon$-$GR_{T}$. If $C$ is assigned to be $1$, there are
$d_0$ possible assignments of $C$ as the same as above, otherwise,
the only possible assignments of $C$ is setting all to $0$.

If $C$ exists in some previous cutting nodes, but its value is not
fixed in $\epsilon$-$GR_{T}$. So $C$ appeared as unfixed in at least
one subtrees. Without losing the generality, we assume that $C$
exists in subtrees $T_{1}, T_{2}\cdots T_{e_0}$, where $e_0\geq 1$,
so there are $d_0 - e_0 + 1\leq d_0$ possible assignments of $C$,
the first assignments set all to $0$, and the $i(\geq 2)$-th
assignments set the value of $C$ in subtree $\mathcal{T}_{i + e_0 -
1}$ to $1$ and rests are $0$.

Since there are at most $(1-\epsilon)\tw(\phi)$ unfixed values in
$p$, so the number of different combinations of
$\epsilon$-$GR_{\mathcal{T}_i}$ which is consistent with
$\epsilon$-$GR_{\mathcal{T}}$ is at most $d^{(1-\epsilon)\tw(\phi)}$

\end{proof}

\subsection {Proof of Lemma \ref{lem:2d-hybrid}}

\begin{proof}
When cutting a $type_{1}$ tree, we pick the cutting node as root,
then cut at the $1 - \alpha$ cutting node, which will result in many
$type_{1}$ trees with size at most $(1 - \alpha)N$ and one
$type_{2}$ tree with size at most $\alpha N$, so we have
\begin{eqnarray*}
T_{1}(N) &\leq& O(d^{(1-\epsilon)\tw'(\phi)})\left(T_{1}\left((1 -
\alpha)N\right) + T_{2}\left(\alpha N\right)\right) +
2^{O(\tw'(\phi))}
\end{eqnarray*}
When cutting a $type_{2}$ tree, suppose the two cutting nodes are
$p_1$ and $p_2$, pick $p_1$ as root and compute the $1/2$-cutting
node $m$. If $m$ is on the path between $p_1$ and $p_2$, cut at $m$,
which will result in two $type_{2}$ trees with size at most $N / 2$
and several $type_{1}$ trees. If $m$ is not on the path between
$p_1$ and $p_2$, we cut at the common ancestor $c$ of $m$ and $p_2$,
while also result in two $type_{2}$ trees with size at most $N / 2$
and several $type_{1}$ trees. So we have
\begin{eqnarray*}
T_{2}(N) &\leq& O(d^{(1-\epsilon)\tw'(\phi)})\left(T_{1}(N) +
T_{2}(N / 2)\right) + 2^{O(\tw'(\phi))}
\end{eqnarray*}
\end{proof}

\subsection {Proof of Theorem \ref{the:2d-time-complexity}}

\begin{proof}
Set $\alpha = \frac{3-\sqrt{5}}{2}$, we have
\begin{eqnarray*}
T_{1}(N) &\leq& O(d^{(1-\epsilon)\tw'(\phi)})\left(T_{1}\left((1 -
\alpha)N\right) + T_{2}\left(\alpha N\right)\right) +
2^{O(\tw'(\phi))}\\
&\leq& O(d^{(1-\epsilon)\tw'(\phi)})T_{1}\left((1 - \alpha)N\right)
+ O(2^{2(1-\epsilon)\tw'(\phi)})T_{1}\left(\alpha N\right) +
2^{O(\tw'(\phi))}
\end{eqnarray*}
According to the Master Theorem, we have
\begin{eqnarray*}
T_{1}(N) &\leq&
O^{*}(d^{\frac{1}{-\log{(1-\alpha)}}(1-\epsilon)\tw'(\phi)\log N})
\end{eqnarray*}
And space requirement is $$O^{*}(2^{2\epsilon\tw'(\phi)})$$
\end{proof}

\subsection {Proof of Theorem \ref{the:worst_case_bound_simple}}

\begin{figure}
\centering{\includegraphics[height=120pt]{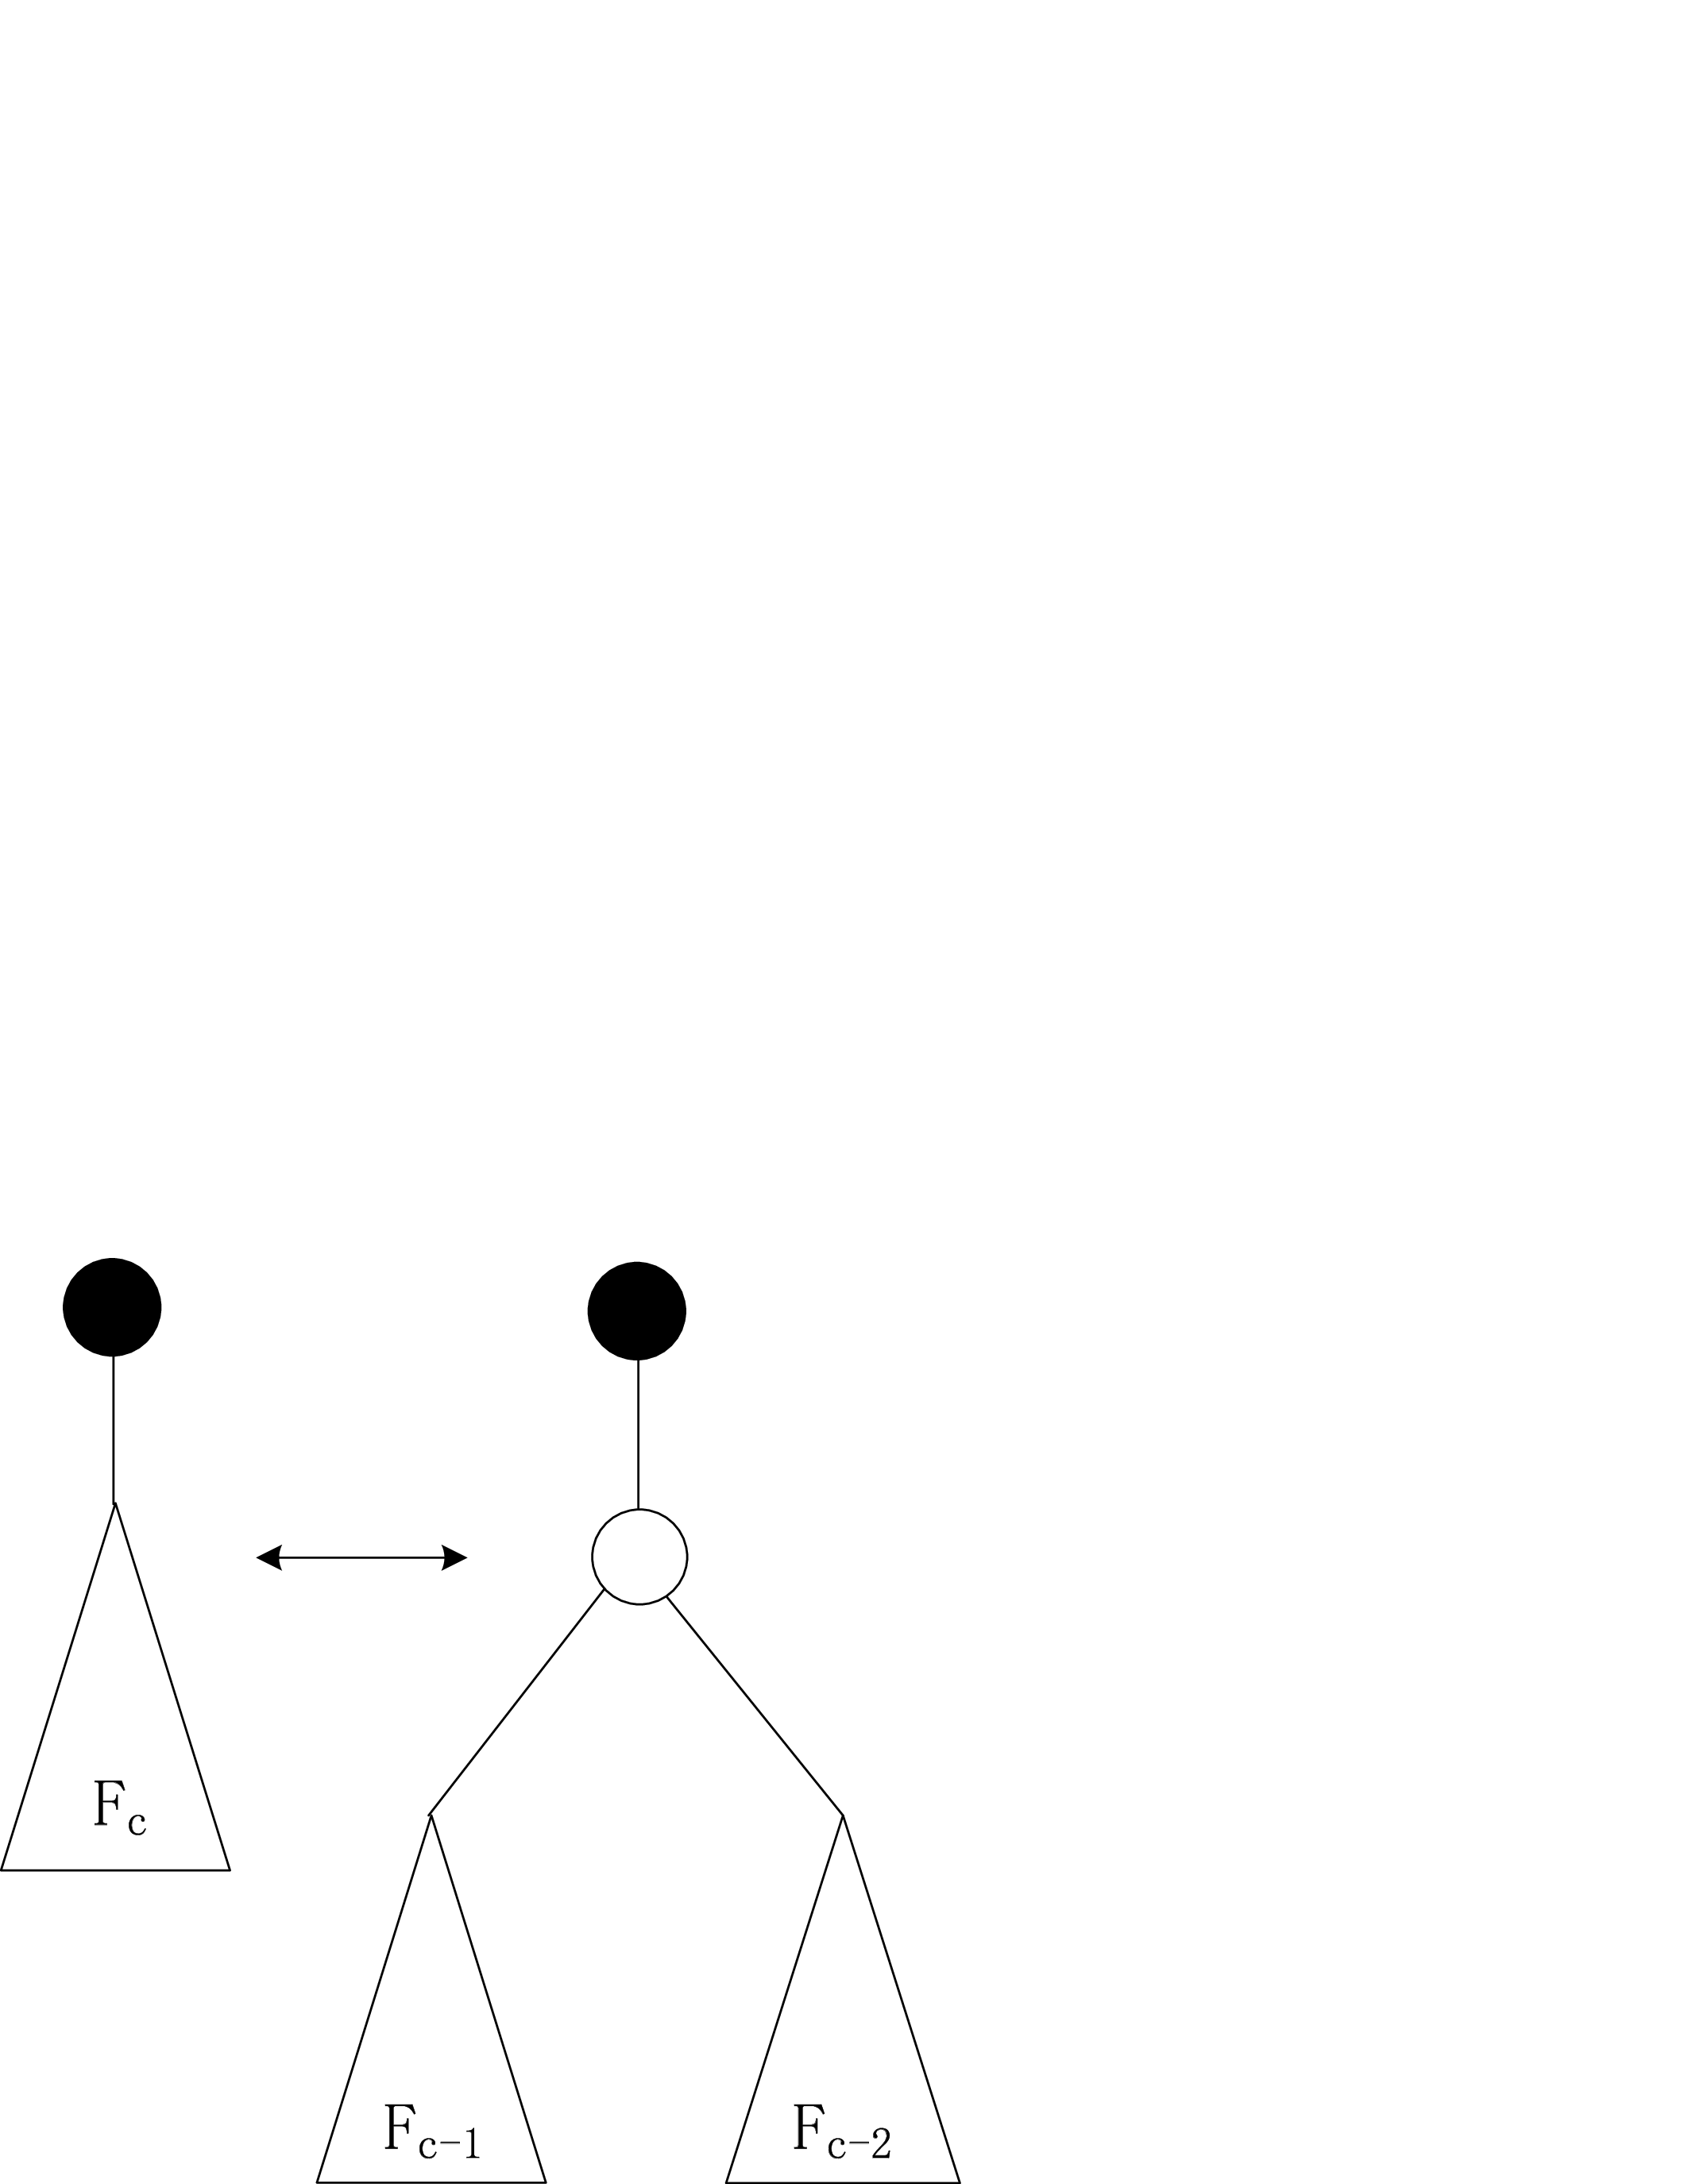}}
\hspace{40pt}{\includegraphics[height=120pt]{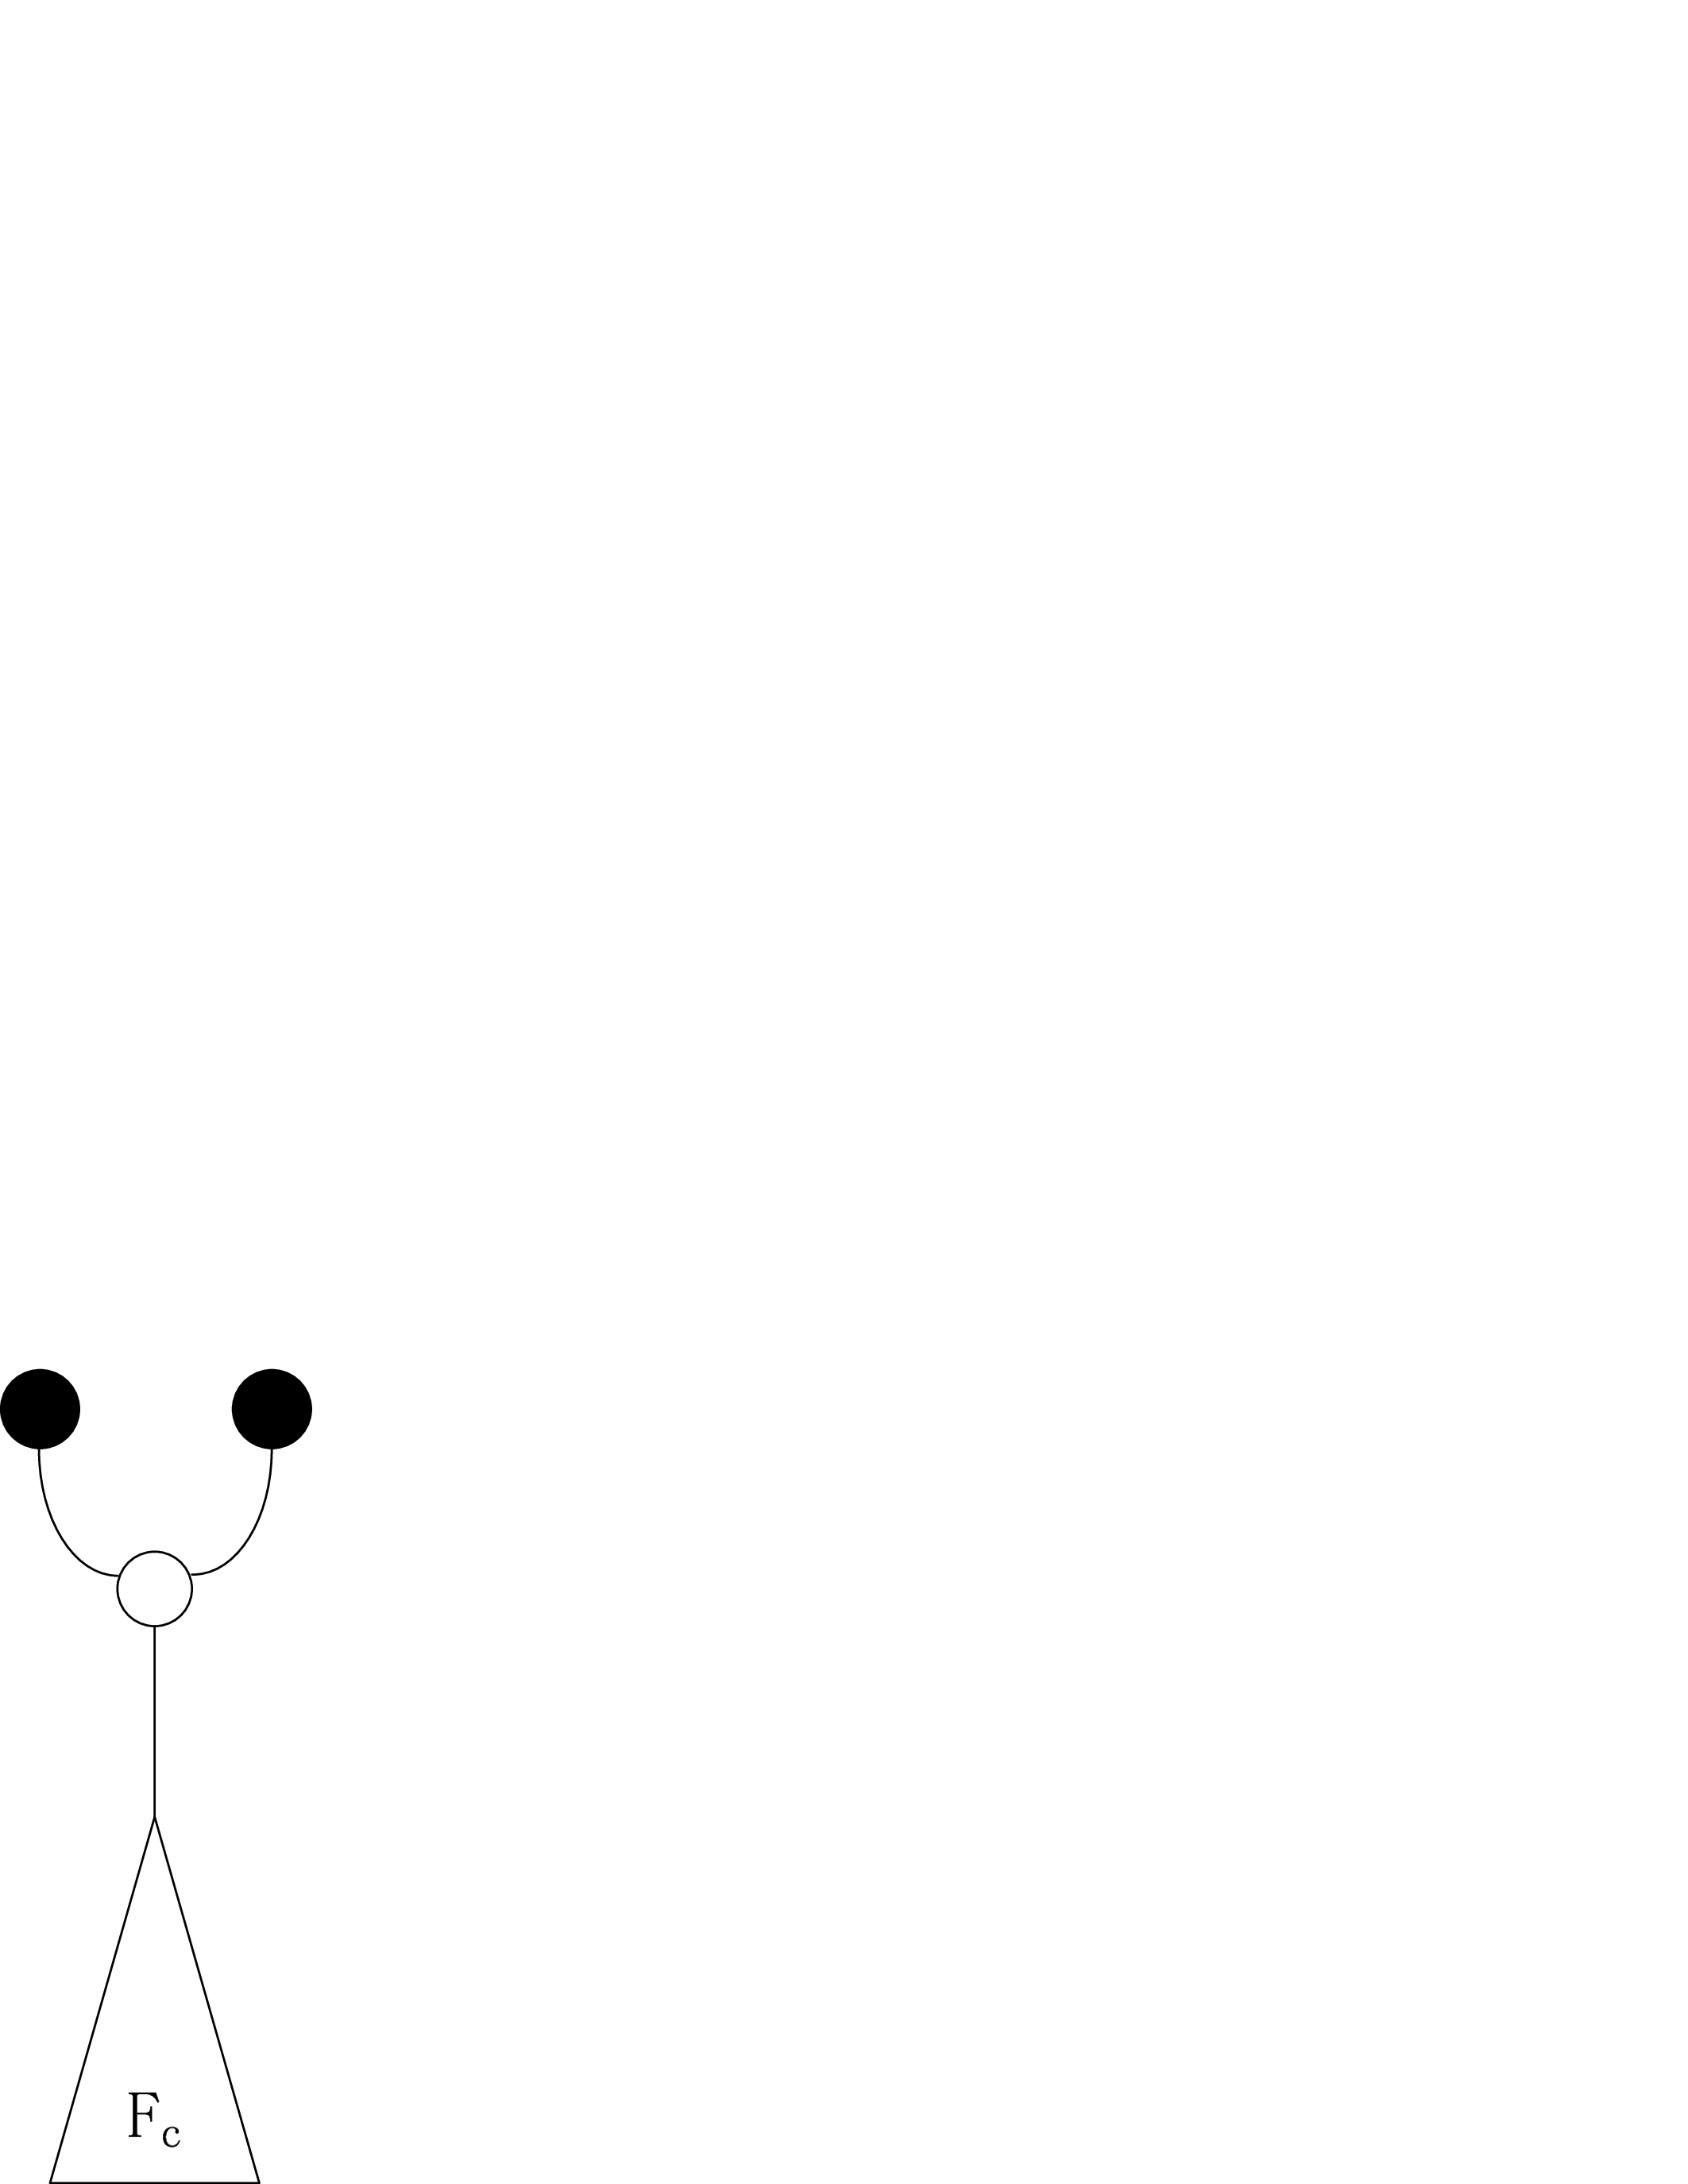}}
\caption{Illustration of two cases for the proof of Theorem
\ref{lem:worst_case_bound_simple_prev}.}\label{fig:worst_case_proof_simple}
\end{figure}

Before proving Theorem \ref{the:worst_case_bound}, we define two
special $type_{1}$ and $type_{2}$ trees as $\mathcal{T}_{1,h}$ and
$\mathcal{T}_{2,h}$. $\mathcal{T}_{1,h}$ tree construct by one
cutting node connect to subtree $F_{h}$, and $\mathcal{T}_{2,h}$
tree construct by two cutting nodes connect to another node which
has subtree $F_{h}$. Now we have the following lemma.

\begin{lemma}\label{lem:worst_case_bound_simple_prev}
The lower bound of processing time for tree $\mathcal{T}_{1,h}$ is
$\Omega^{*}(d^{(1-\epsilon)\tw'(\phi)h})$, and for tree
$\mathcal{T}_{2,h}$, the lower bound is
$\Omega^{*}(d^{(1-\epsilon)\tw'(\phi)(h + 1)})$.
\end{lemma}

\begin{proof}
We prove by induction. It is easy to prove the case when $h\leq 2$.
Suppose the lemma is correct for any $h_0 < h$. For tree
$\mathcal{T}_{1,h}$, if we cut at the root of $F_h$, the processing
time is at least $\Omega^{*}(d^{(1-\epsilon)\tw'(\phi)(1 + (h -
1))})$, if we cut at subtrees $F_{h-1}$ or $F_{h-2}$, the processing
time is at least $\Omega^{*}(d^{(1-\epsilon)\tw'(\phi)(1 + (h - 2) +
1)})$. So the lower bound for tree $\mathcal{T}_{1,h}$ is
$\Omega^{*}(d^{(1-\epsilon)\tw'(\phi)h})$. For tree
$\mathcal{T}_{2,h}$, we must cut at the node connecting two cutting
nodes, so the lower bound is $\Omega^{*}(2^{(1-\epsilon)\tw'(\phi)(1
+ h)})$.
\end{proof}

\begin{proof}
Set $\alpha = \frac{3-\sqrt{5}}{2}$, since the number of nodes in
$F_h$ is $O({\frac{1+\sqrt{5}}{2}}^{h})$, we have a lower bound for
running time
$\Theta^{*}(d^{\frac{1}{-\log{(1-\alpha)}}{(1-\epsilon)\tw'(\phi)\log
N}})$. And the previous bound is tight.
\end{proof}

\subsection {Proof of {Lemma} \ref{lem:algorithm_complexity}}
\begin{proof}
When $N\geq 2^{c}$, for each $1\leq i<c$, when we want to cut a
$type_{i}$ tree with cutting nodes $|S| = i$, we first pick one
cutting point as root.

Then compute a $(1 - \alpha_{c, i})$-cutting-node $m$ in this tree.
If $m$ is not on the path between any pairs of previous cutting
points, we cut at $m$, which will result in many $type_{1}$ trees
with size at most $\lceil{(1 - \alpha_{c, i})N}\rceil$ and one
$type_{i + 1}$ trees with size at most $\lceil{\alpha_{c,
i}N}\rceil$. Otherwise, since $1 - \alpha_{c, i} > 1 / 2$, it
implies that, the maximal possible size of $type_{1}$ tree can be
cut by any cutting point does not exceed $\lceil{(1 - \alpha_{c,
i})N}\rceil$. Then, we compute a $1/2$-cutting-node $c$ in this
tree. If $c$ is on the path between some pairs of previous cutting
points, we cut at $c$
 which will result in many $type_{j}(j\leq i)$ trees
with size at most $\lceil{N/2}\rceil$, otherwise, we compute the
least common ancestor of $c$ and all previous cutting nodes as $p$,
and cut at $p$ which be cut in many $type_{1}$ tree with size at
most $\lceil{(1 - \alpha_{c, i})N}\rceil$ and many $type_{j}(j\leq
i)$ trees with size at most $\lceil{N/2}\rceil$.

Therefore, we have $$D_{c,i}(N) = \max\{D_{c,1}\left((1 - \alpha_{c,
i})N\right), D_{c,i + 1}\left(\alpha_{c, i}N\right), D_{c,i}\left(N
/ 2\right) \} + 1$$.

When we want to cut a $type_{c}$ tree with cutting nodes $|S| = c$,
since $\alpha_{c, c} = 0$, we always ignore the $(1 - \alpha_{c,
i})$-cutting-node $m$, then we compute the $1/2$-cutting-node $c$.
If $c$ is on the path between some pairs of previous cutting points,
we cut at $c$
 which will result in many $type_{j}(j\leq i)$ trees
with size at most $\lceil{N/2}\rceil$, otherwise, we compute the
least common ancestor of $c$ and all previous cutting nodes as $p$,
and cut at $p$ which be cut in many $type_{1}$ tree with size at
most $N$ and many $type_{j}(j\leq i)$ trees with size at most
$\lceil{N/2}\rceil$. Therefore, we have $$D_{c, c}(N) = \max\{D_{c,
1}(N) + D_{c, c}(N / 2)\} + 1$$.
\end{proof}

\subsection {Proof of {Lemma}
\ref{lem:algorithm_complexity2}}
\begin{proof}

When $N\geq 2^{c}$, for each $c\geq 2$, $1\leq i<c$, we have
$$D_{c,i}(N)=\max\{D_{c,1}((1-\alpha_{c, i}) N), D_{c,i+1}(\alpha_{c, i}N),
D_{c,i}(N/2)\} + 1$$ and $$D_{c,c}(N)=\max\{D_{c,1}(N),
D_{c,c}(N/2)\} + 1$$

For each $1\leq i\leq c$, $D_{c,i}(N)\geq D_{c,i}(N/2) + 1$. So we
get
$$D_{c,i}(N)=\max\{D_{c,1}((1 - \alpha_{c, i}) N), D_{c,i + 1}(\alpha_{c, i}N)\}
+ 1$$ and $$D_{c,c}(N)=D_{c,1}(N) + 1$$

Furthermore, for each $1<i\leq c$, since $D_{c,1}((1-\alpha_{c, i})
N) = D_{c,i + 1}( \alpha_{c, i}N)$, we have $$D_{c,i}(N) =
D_{c,1}((1 - \alpha_{c, i - 1})N /\alpha_{c, i - 1})$$

For each $1\leq i< c$, since $D_{c,i}(N) = D_{c,1}((1 - \alpha_{c,
i})N) + 1 $, on the other hand, $D_{c,i}(N) = D_{c,i+1}(\alpha_{c,
i}N) + 1 = D_{c,1}(\alpha_{c, i}(1 - \alpha_{c, i + 1})N) + 2$, so
we get
$$D_{c,1}(N) = D_{c,1}(\alpha_{c, i}(1 - \alpha_{c, i + 1}) / (1 - \alpha_{c, i})N) +
1$$ Since $D_{c,1}(N) = D_{c,1}((1 - \alpha_{c, 1})N) + 1$, we have
$(1 - \alpha_{c, 1})(1 - \alpha_{c, i})N = \alpha_{c, i}(1 -
\alpha_{c, i + 1})$, and $\alpha_{c, i + 1} = 1 - (1 - \alpha_{c,
1})(1 - \alpha_{c, i})/\alpha_{c, i}$. Therefore, we have
$$\alpha_{c, i} = 1 - \frac{\alpha_{c, 1}(1-\alpha_{c, 1})^{i}}{2\alpha_{c, 1} -
1 + (1 - \alpha_{c, 1})^{i}}$$

On the other hand, $D_{c,c}(N) = D_{c,1}(N) + 1 = D_{c,1}((1 -
\alpha_{c, c-1})N/\alpha_{c, c-1})$, so we have $\alpha_{c, c-1}/(1
- \alpha_{c, c}) = 1 - \alpha_{c, 1}$ and $\alpha_{c, c-1} = (1 -
\alpha_{c, 1})/(2 - \alpha_{c, 1})$. Thus, we have $(1 - \alpha_{c,
1})/(2 - \alpha_{c, 1}) = 1 - \frac{\alpha_{c, 1}(1-\alpha_{c,
1})^{c - 1}}{2\alpha_{c, 1}- 1 + (1 - \alpha_{c, 1})^{c - 1}}$ , so
we get
$$\sum_{i=1}^{c}(1 - \alpha_{c, 1})^{i} = 1$$.

Since $D_{c,1}(2^c) = c$, we set $\lambda_{c} = \frac{1}{\log (1 -
\alpha_{c, 1})}$, the $c$-cutting depth of a tree with $N$ nodes by
the algorithm $\mathcal{A}$ is $\lambda_{c}(\log N - c) + c + O(1)$,
where $\lambda_{c}$ satisfied
$\sum_{l=1}^{c}2^{-\frac{l}{\lambda_{c}}} = 1$

\end{proof}

\subsection {Proof of Theorem~\ref{the:algorithm_complexity}}
\begin{proof}
For any $c \geq 2$, according to the Master Theorem, when $N <
2^{c}$, the running time is,
$$O^{*}\left(d^{\log N (1-\epsilon)\tw'(\phi)}\right)$$
So, when $N > 2^{c}$, the running time is
$$O^{*}\left(d^{\left(\lambda_{c}(\log N - c) + c\right) (1-\epsilon)\tw'(\phi)}\right)$$, and
the space is no more than $$O^{*}(2^{c\epsilon\tw(\phi)})$$
\end{proof}

\subsection {Proof of {Lemma} \ref{lem:worst_case_bound}}

Before proving {Lemma} \ref{lem:worst_case_bound}, we have the
following definition. For any $c\geq 2$, $h > c$ and $1 \leq h \leq
c$, we define tree $G_{c, h, w}$ as following, we first construct a
chain of length $w$, and $c - w + 1$ cutting nodes connect to the
first node of the chain, the $i$-th node of the chain have a subtree
$F_{c, h - c + w - i}$. We denote $S_{\ell}$ as the set of the
$\ell$ cutting nodes connect to the first node of the chain.
Specifically, $MCD_{c}(F^{*}_{c, h, r},\{r\}) = MCD_{c}(G_{c, h, c},
S_{1})$.  We have the following lemma.
\begin{lemma}\label{lem:prev_worst_case_bound}
$MCD(G_{c, h, w}, S_{c - w + 1})\geq h - c + w$
\end{lemma}

\begin{proof}
We prove {Lemma} \ref{lem:prev_worst_case_bound} and Lemma
\ref{lem:worst_case_bound} by induction. When $h \leq c$,
$MCD_(G_{c, h, c}, S_{1}) = MCD_c(F^{*}_{c, h, r}, \{r\}) \geq h$.

Suppose for each $h_{0} < h(h > c)$, we have $MCD_c(G_{c, h_{0}, c},
S_{1}) = MCD_c(F^{*}_{c, h_{0}, r}, \{r\}) \geq h_{0}$.

If $w = 1$, in order to get rid of exceeding $c$ cutting node in one
subtree, we must cut at the first node of the chain, so we have
$MCD_{c}(G_{c, h, 1}, S_{c}) = 1 + MCD_{c}(F^{*}_{c, h - c, r},
\{r\}) = 1 + MCD_{c}(G_{c, h - c, c}, S_{1}) \geq h - c + 1$.

When $w > 1$, if we cut on the subtree $F_{c, h - c + w - 1}$
connected to the first node of the chain, we have
\begin{eqnarray*}
MCD_{c}(G_{c, h, w}, S_{c - w + 1}) &=& 1 + MCD_{c}(G_{c, h, w - 1},
S_{c - w + 2})\\
& \geq & 1 + (h - c + (w - 1))\\
& = & h - c + w
\end{eqnarray*}, otherwise, we have
\begin{eqnarray*}
MCD_{c}(G_{c, h, w}, S_{c - w + 1}) &=&  1 + MCD_{c}(G_{c, h - c + w
- 1, c}, S_{1}) \\
&=& h - c + w
\end{eqnarray*}
\end{proof}

\begin{figure}
\centering{\includegraphics[height=200pt]{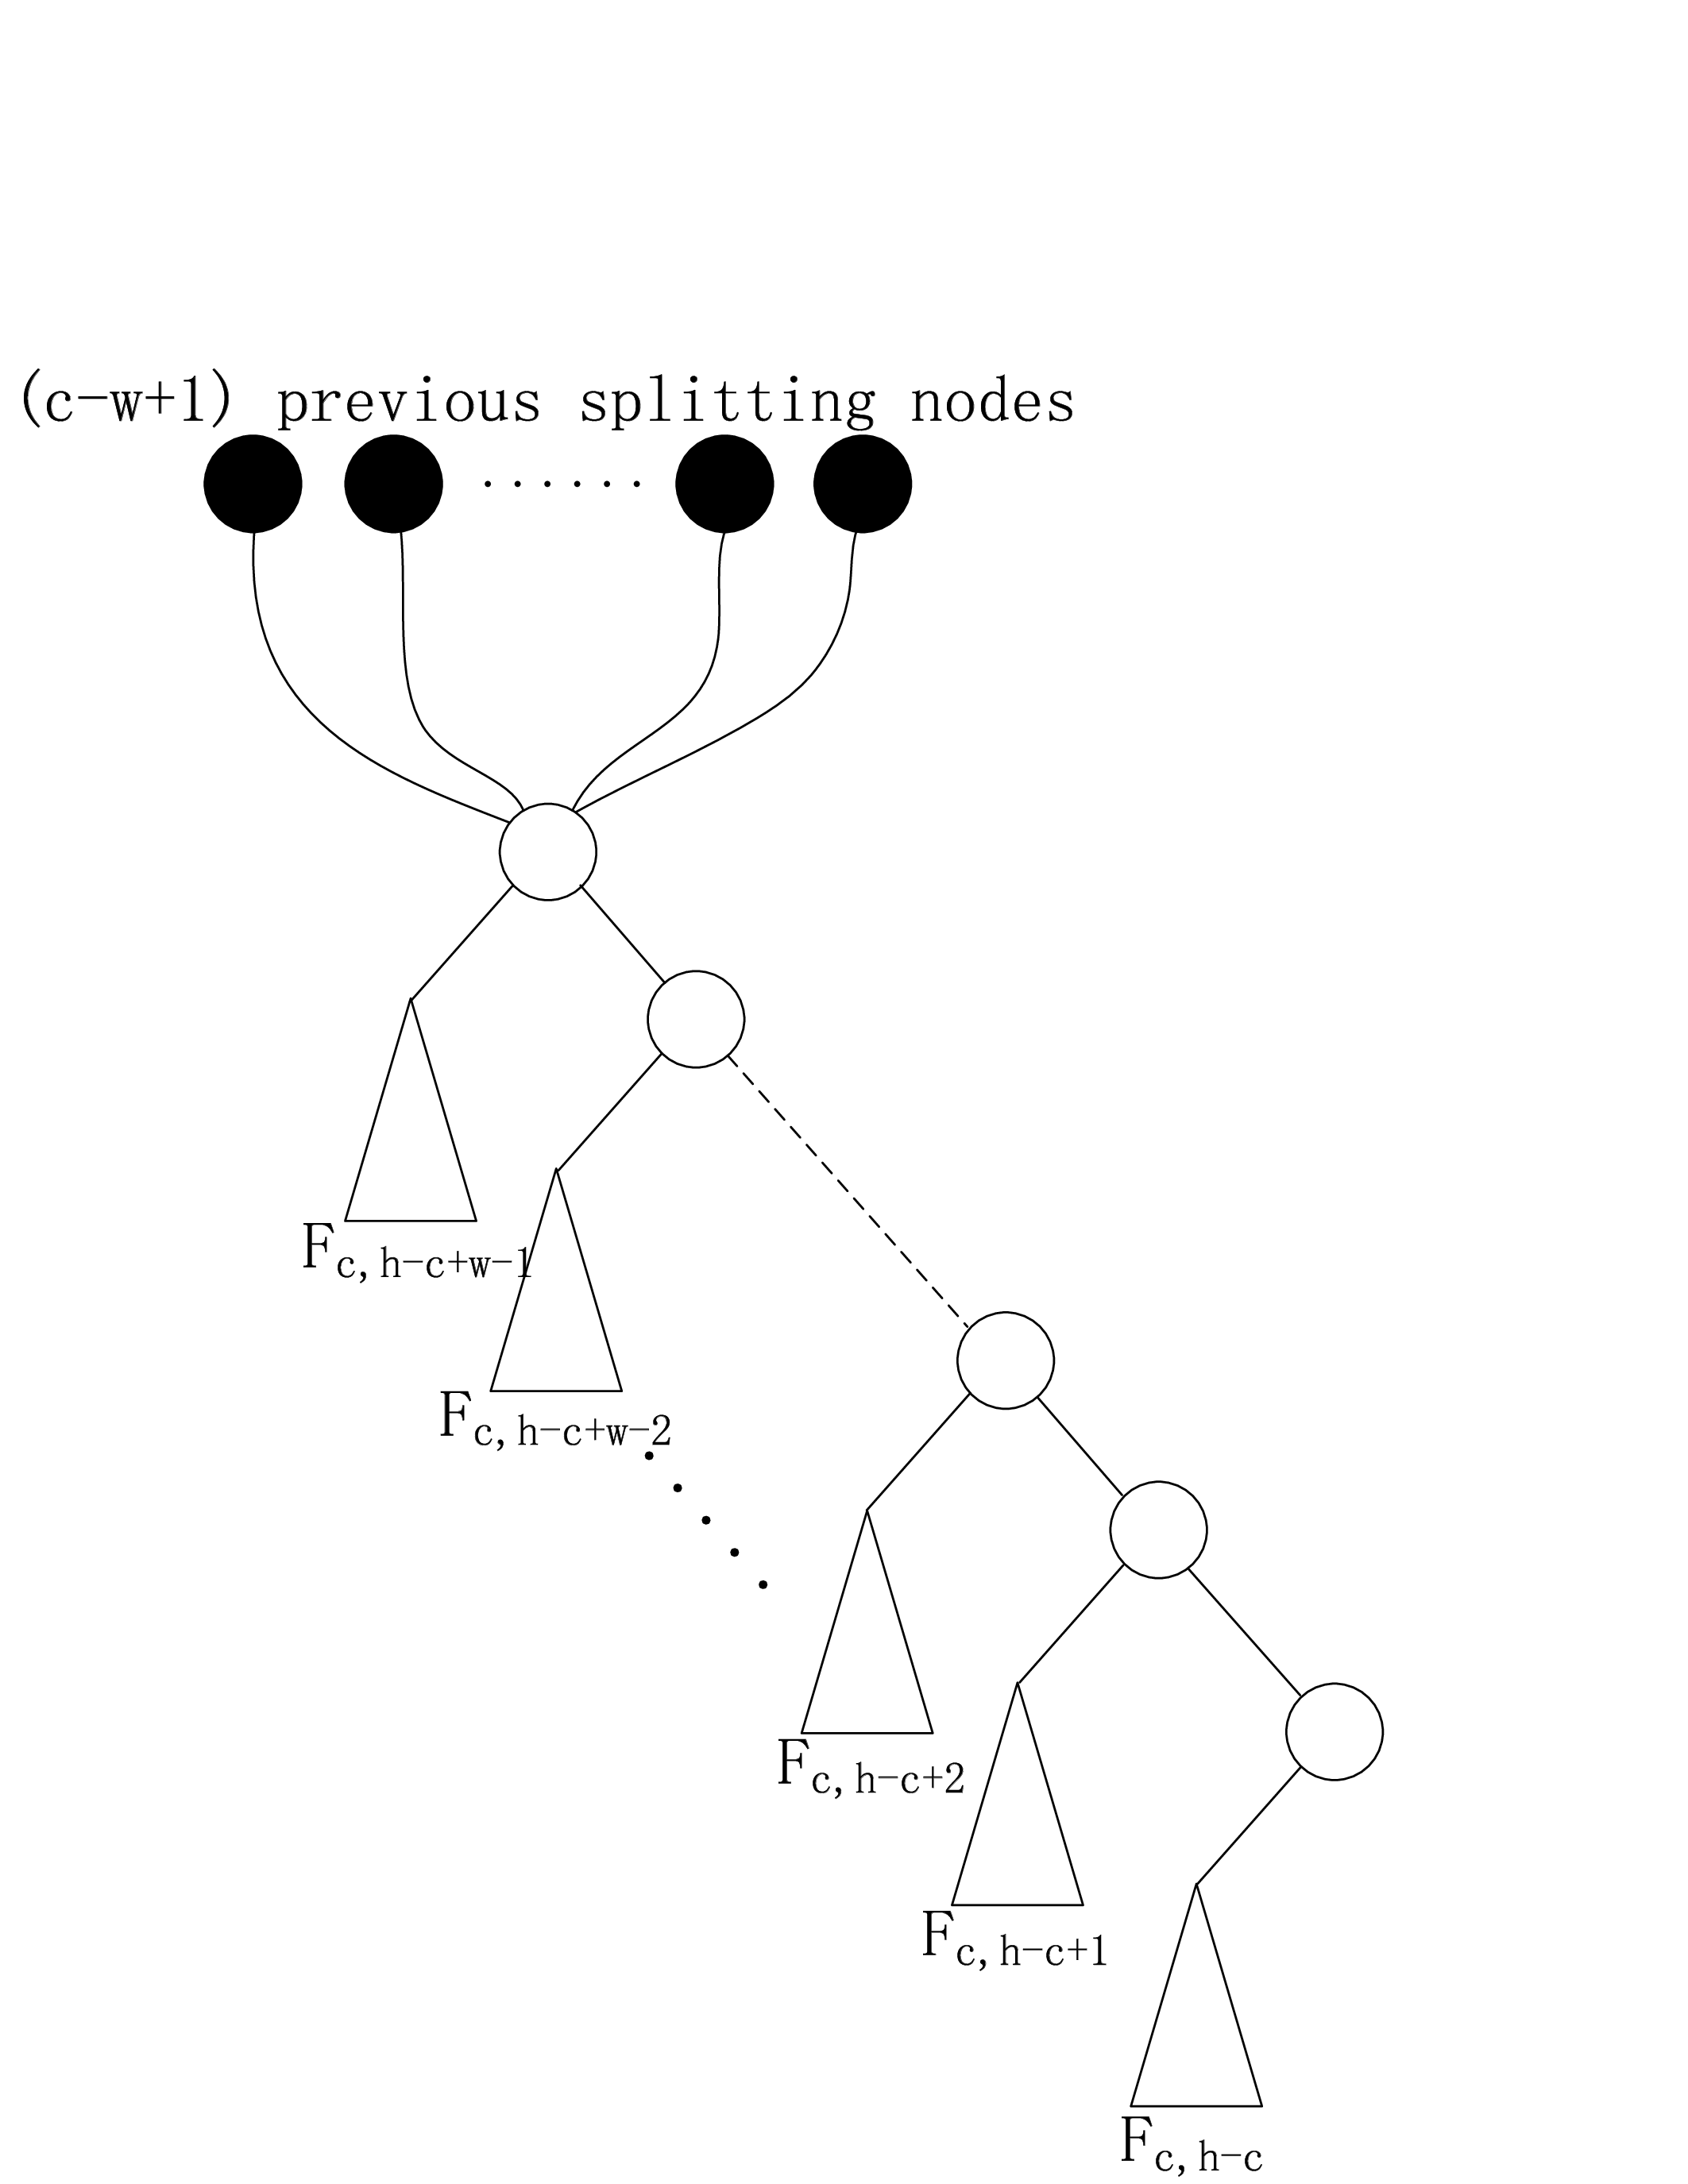}}
\caption{Illustration of tree $G_{c, h,
w}$.}\label{fig:worst_case_proof}
\end{figure}

\subsection {Proof of {Theorem} \ref{the:worst_case_bound}}
\begin{proof}
We use $|F_{c, h}|$ to denote the number of nodes in the tree $F_{c,
h}$. For any $h\leq c$, we have $|F_{c, h}|\leq 2^{c}$, when $h
> c$, we have $|F_{c, h}| = \sum_{i = 1}^{c}|F_{c, h - i}| + c$. By
generating function of $|F_{c, h}|$, we have $|F_{c, h}| = \sum_{i =
1}^{c}{\delta_{c, i}\gamma_{c, i}^{h - c}}$. The $\delta_{c,i} =
O(2^{c})$ and $\gamma_{c, i}$ is the $i$-th root of the equation
$X^{c} - \sum_{i=0}^{c}{X^{i}} = 0$.

Suppose the $\gamma_{c}$ is the root with largest absolute value.
When $h$ is larger, we have $|F_{c, h}| = \Theta(2^{c}\gamma_{c}^{h
- c})$. So, $h \geq \log_{\gamma_{c}}{\left({|F_{c, h}| /
2^{c}}\right)} + c - O(1) = \lambda_{c}(\log_{|F_{c, h}|} - c) + c -
O(1)$. Therefore, for any $c\geq 2$ and $N > 0$, there exists a tree
$\mathcal{T}$ with at most $N$ nodes, such that the $c$-minimal
cutting depth of $\mathcal{T}$ ($MCD(\mathcal{T}, \emptyset)$) is at
least $\lambda_{c} (\log N - c) + c - O(1)$.
\end{proof}

\subsection{Proof of Corollary~\ref{cor:hybrid_opt_space}}
Before proving Corollary~\ref{cor:hybrid_opt_space}, we need to proof 2 lemmas first.
\begin{lemma}\label{lem:bound_of_gamma}
$\gamma_{c}>2-\frac{1}{2^{\frac{c}{2}}}$
\end{lemma}
\begin{proof}
suppose $f(X)=X^{c}-\sum_{i=0}^{c}{X^{i}}$ then $\gamma_{c}$ is the
root of $f(X)=0$ with largest absolute value We know $f(2)=1>0$, so
if we can proof $f(2-\frac{1}{2^{\frac{c}{2}}}<0)$ then there is a
root between 2 and $2-\frac{1}{2^{\frac{c}{2}}}$. Suppose
$y=2-\frac{1}{2^{\frac{c}{2}}}$
\begin{eqnarray*}
f(y)<0&\iff& y^{c}<\sum_{i=0}^{c}{y^{i}}=\frac{y^{c}-1}{y-1}\\
&\iff& y<2-\frac{1}{y^c}
\\&&\textrm{Because } y=2-\frac{1}{2^{\frac{c}{2}}}>\sqrt{2} \textrm{ when } c\le2
\\&&\textrm{So } 2-\frac{1}{y^c}>2-\frac{1}{\sqrt{2}^{c}}=y
\end{eqnarray*}
\end{proof}
\begin{lemma}\label{lem:bound_of_lambda}
$\lambda_c<1+\frac{1}{2^{\frac{c}{2}}}$
\end{lemma}
\begin{proof}
That is because of $\lambda_c=\frac{1}{\log_{2}{\gamma_{c}}}$ and
$\gamma_{c}>2-\frac{1}{2^{\frac{c}{2}}}$
\end{proof}
And then, the proof of Theorem~\ref{cor:hybrid_opt_space}
\begin{proof}
For a fixed $\epsilon'$, according to
{Theorem}\ref{the:algorithm_complexity} we know there is an
algorithm with running time
$O^*(d^{\lambda_{c}(1-\epsilon)\log_{2}{N}\tw'(\phi)})$ and space
$O^*(2^{c\epsilon\tw'(\phi)})$ for any $\epsilon>0$. Set
$\epsilon=\frac{\epsilon'}{c}$, then the space is
$O^*(2^{\epsilon'\tw'(\phi)})$ and the running time is
$O^*(d^{\lambda_{c}(1-\frac{\epsilon'}{c})\log_{2}{N}\tw'(\phi)})$
According to {Lemma}\ref{lem:bound_of_lambda}, we know
$\lambda_{c}(1-\frac{\epsilon'}{c})<(1+\frac{1}{2^{\frac{c}{2}}})(1-\frac{\epsilon'}{c})<1$
when $c$ is large enough.
\end{proof}

\subsection{Proof of Theorem~\ref{thm:sat_tw}}
$\sat_{tw}(\log^l{n})$ can be solved by a depth-first-search algorithm on the tree decomposition on an $\nauxpda$ using $O(\log^l{n})$ space and polynomial time as shown in \cite{GP08}. The details are omitted here. It follows that $\sat_{tw}(\log^l{n})$ is contained in $\nauxpda(\log^l{n}, poly(n))$.

Now we turn to prove the hardness. By the characterization theorems from \cite{venkateswaran1987properties} and \cite{ruzzo1980tree}, it can be shown that $\nauxpda(\log^l{n},poly(n))\subseteq\sac(2^{O(\log^l{n})}, \log^l{n})$ by $O(\log^l{n})$ space bounded transformations. Now it suffices to construct a $\sat_{tw}(\log^l{n})$ instance $\phi$, given the $\sac(2^{O(\log^l{n})}, \log^l{n})$ circuit $C$ and an input $x$, such that $\phi$ is satisfiable if and only if $C$ evaluates to $1$ on $x$.

The construction and terminology follow \cite{gottlob2001complexity}, which are used to prove the $\logcfl$-hardness of Acyclic Conjunctive Queries problem. W.l.o.g, we assume that the circuit has the following \emph{normal form}:
\begin{enumerate}[(1)]
\item Fan-in of all AND gates is $2$.
\item The circuit is \emph{layered}.
\item The circuit is \emph{strictly alternating}, odd-layer gates are OR, even-layer gates are AND.
\item The circuit has an odd number of layers.
\item NOT gates only appear in the bottom layer.
\end{enumerate}

\begin{figure*}[ht]
\centering \subfloat[A semi-unbounded circuit with a proof tree
highlighted. NOT gates are
hidden]{\includegraphics[height=130pt]{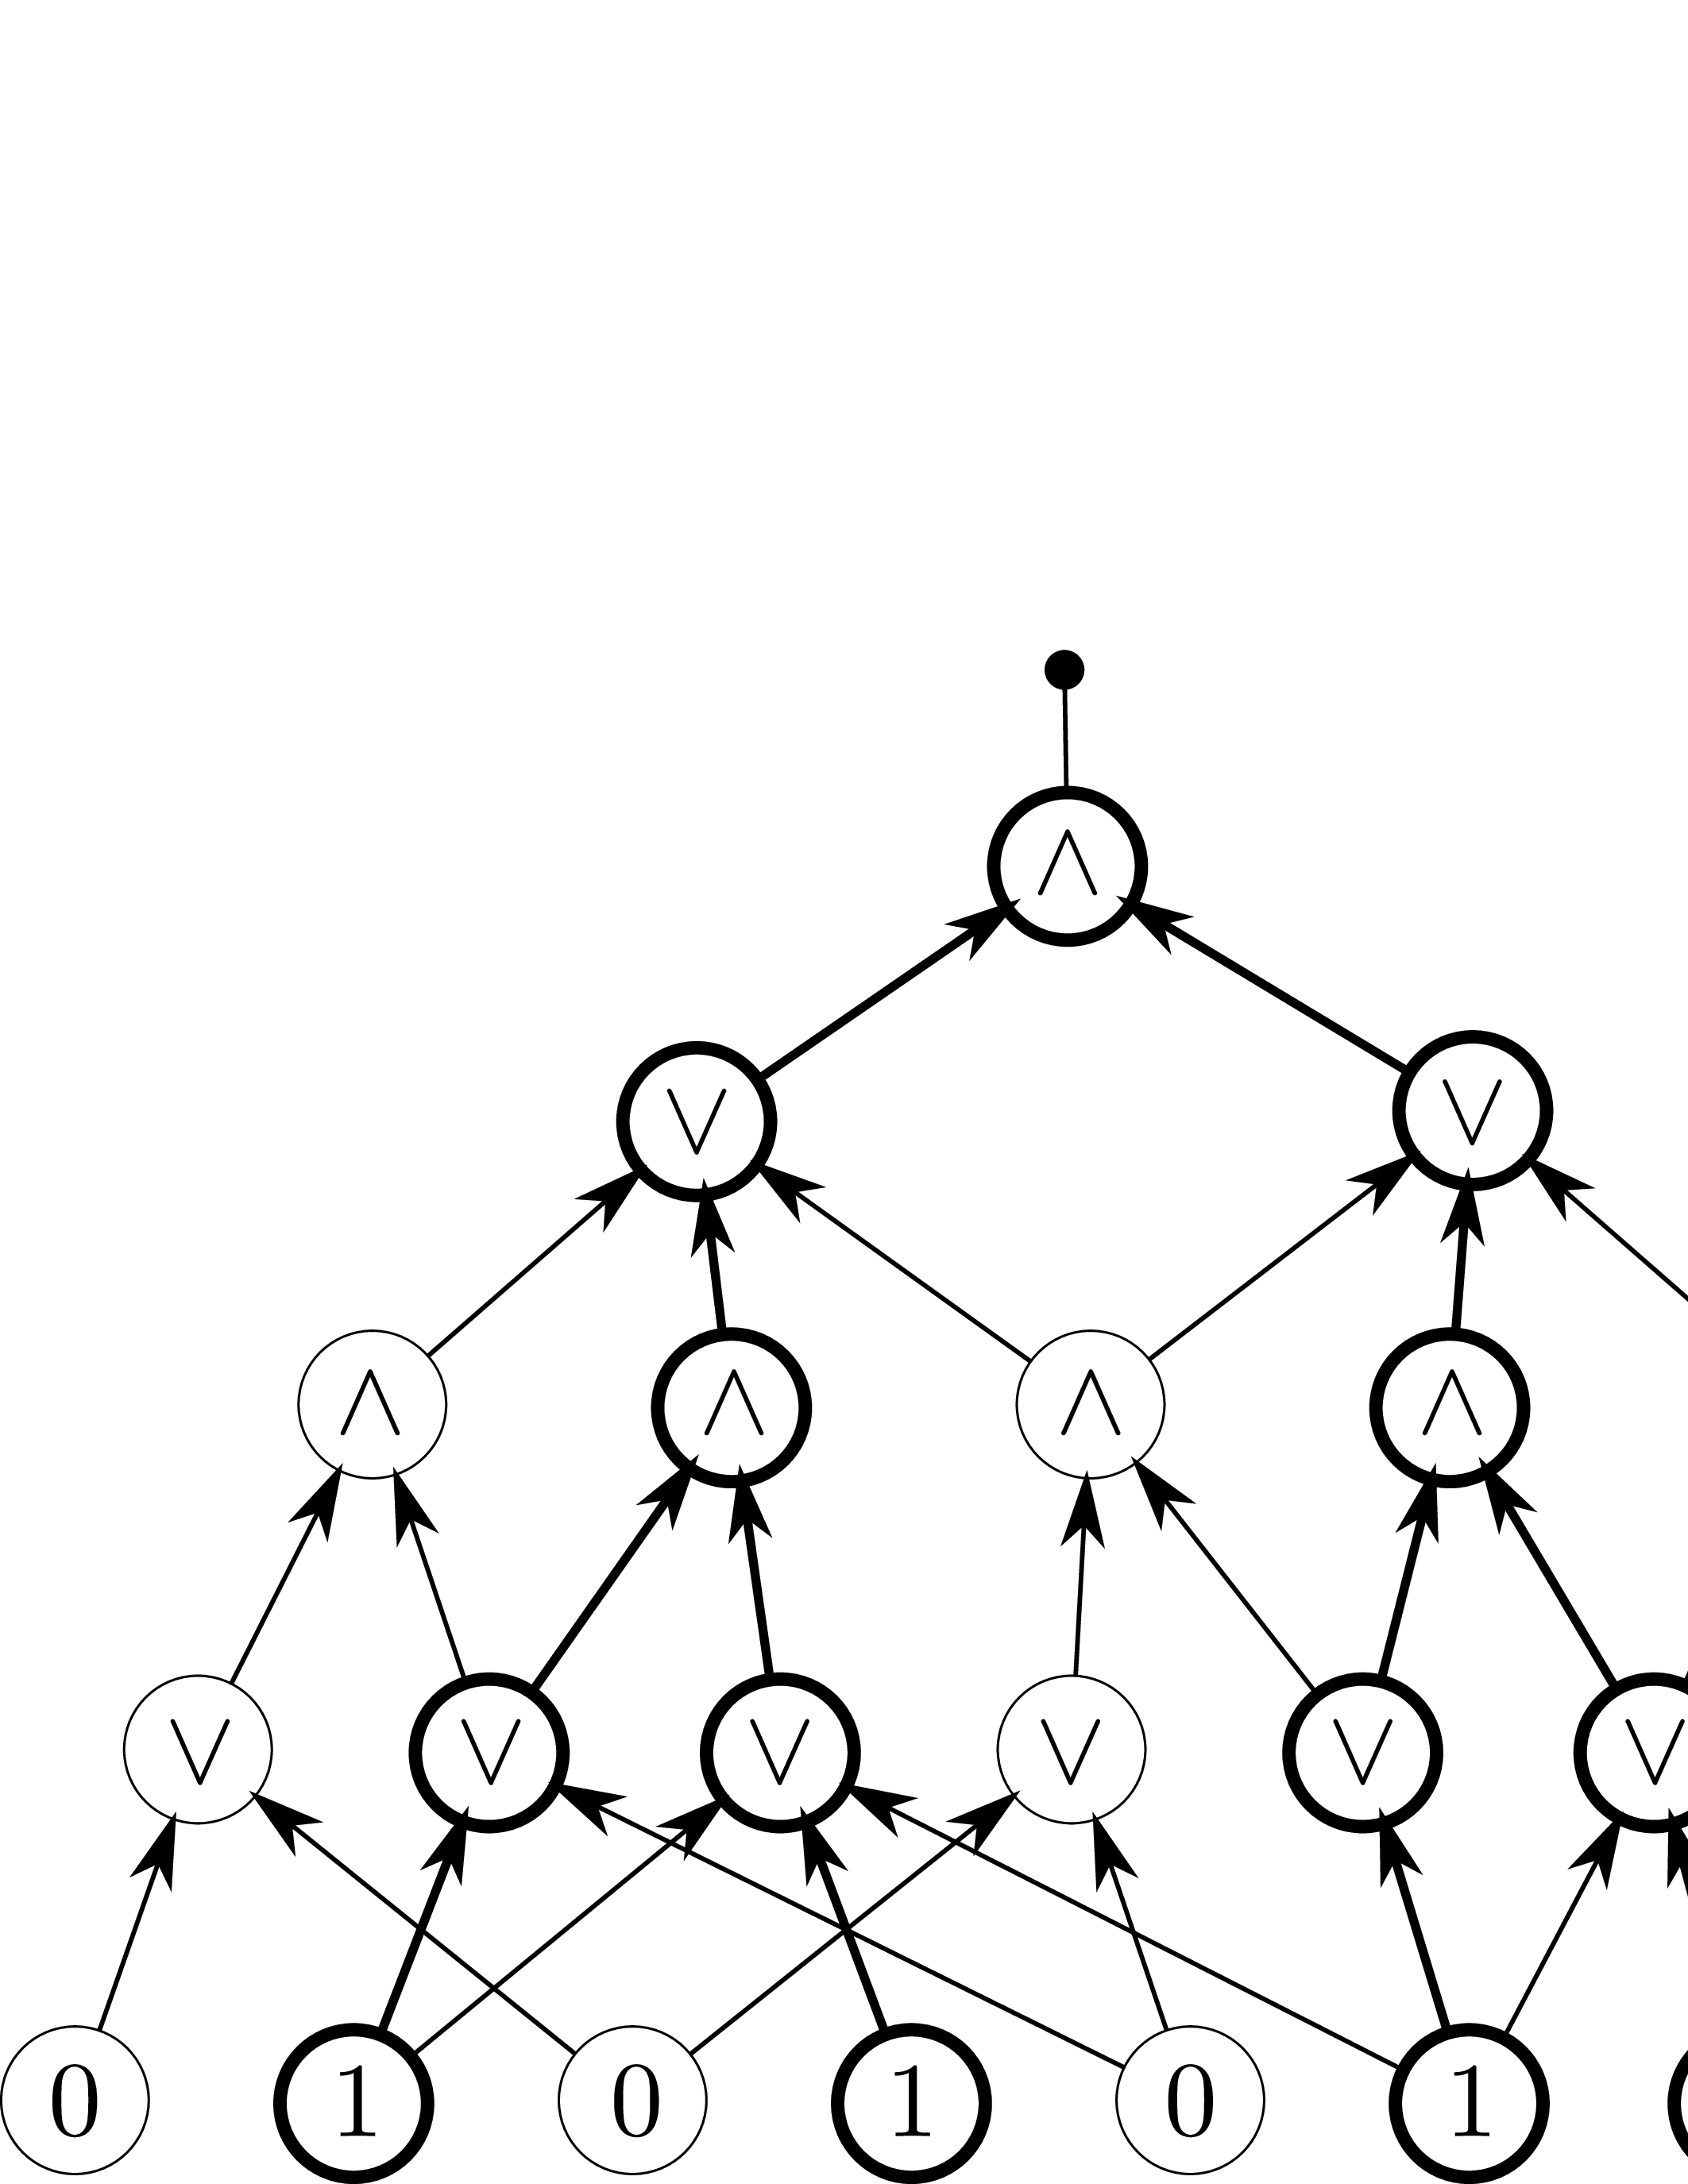}\label{subfig:proof_tree}}
\hspace{40pt} \subfloat[The skeleton of the proof trees]
{\includegraphics[height=130pt]{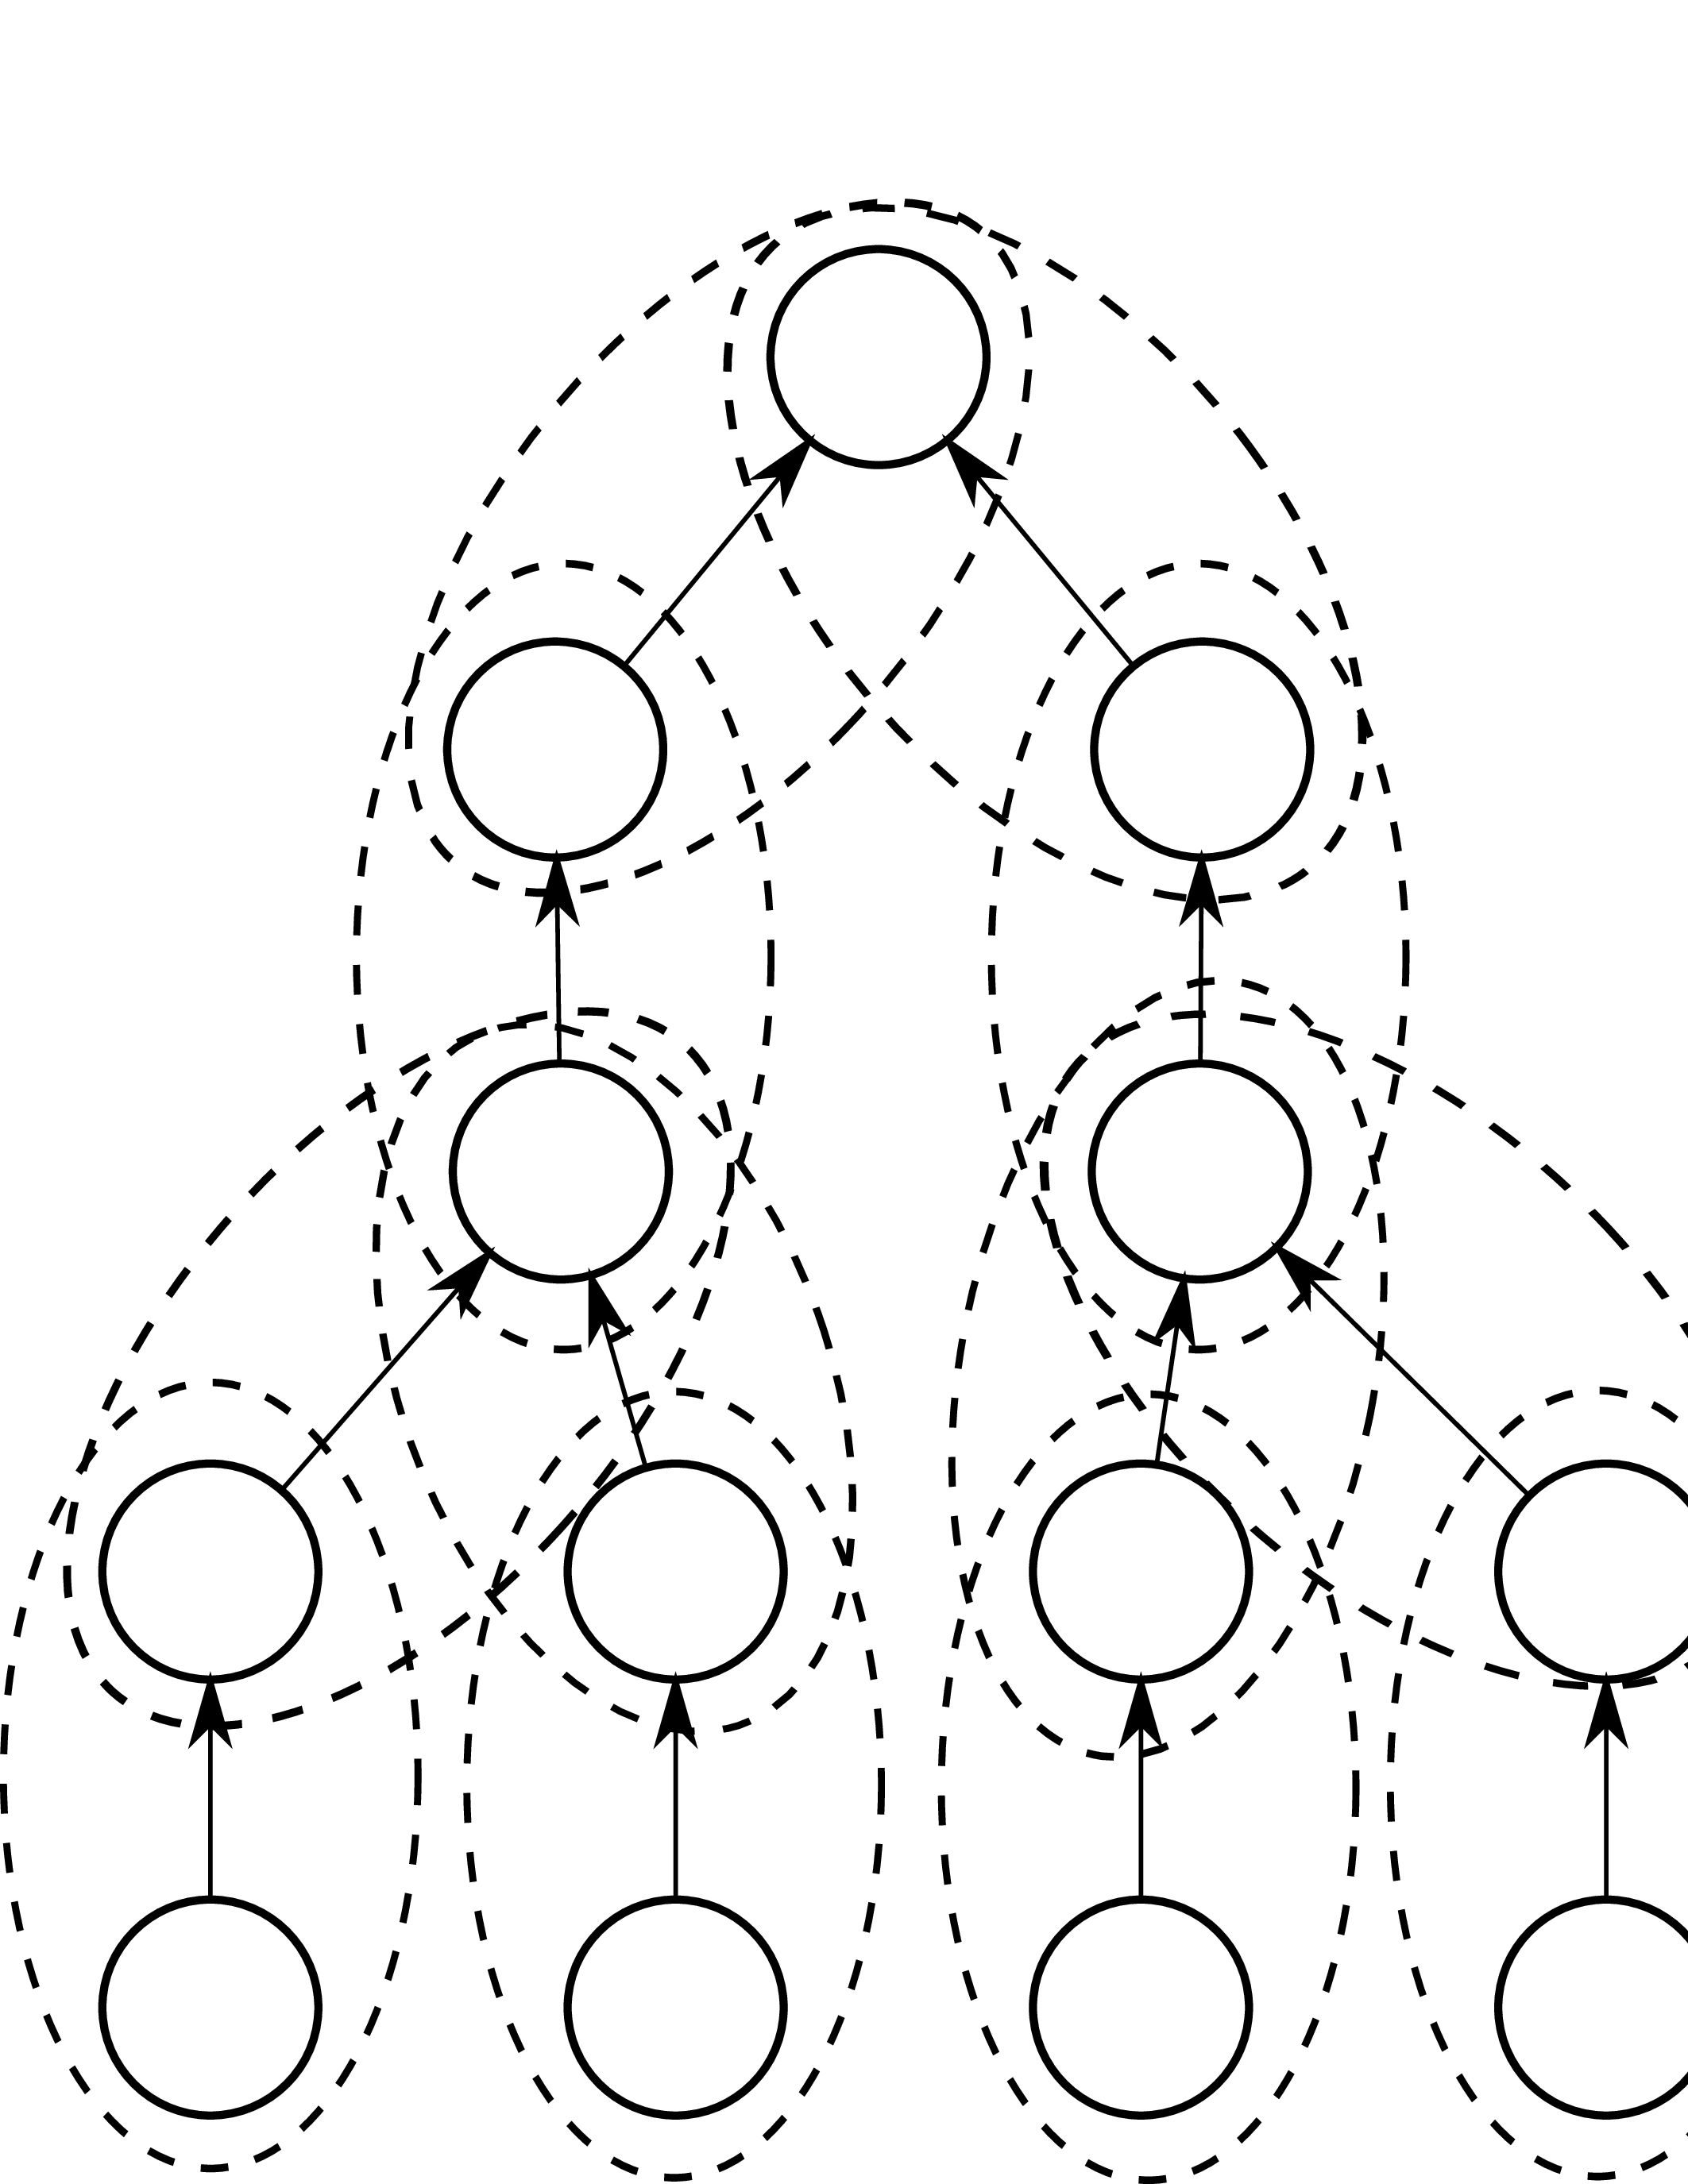}\label{subfig:skeleton}}
\caption{An example adapted from \cite{gottlob2001complexity}. In
\ref{subfig:skeleton} a $\sat_{tw}(\log^l{n})$ instance is
constructed from the skeleton: each node corresponds to
$O(\log^l{n})$ boolean variables; clauses are constructed for each
dashed circle; and only those variables corresponding to a node
shared by different dashed circles must be put into a bag in the
tree decomposition, which ensures $O(\log^l{n})$ tree
width.}\label{fig:logcfl_hard}
\end{figure*}

A \emph{proof tree} is a tree with the same layering as the circuit. Each node of the tree is labeled by a gate from the corresponding layer of the circuit. At an odd layer, each node has one child, while at an even layer, each node has two children. Two connected nodes must be labeled such that the corresponding gates are connected. At the bottom layer, each node must be labeled by an input gate or a NOT gate which outputs value $1$. See Figure~\ref{subfig:proof_tree} for an example.

A proof tree can be viewed as the witness that a circuit evaluates to $1$ on the given input. One may observe that, since we assume that all the circuits are of normal form, every proof tree must have the same shape. The tree of the same shape of a proof tree without labeling is called a \emph{skeleton}(Figure~\ref{subfig:skeleton}). Showing that the circuit evaluates to $1$ on an input is equivalent to giving a labeling satisfying the proof tree conditions to the skeleton.

One of the $2^{O(\log^l{n})}$ gates in the circuit can be indexed by a $O(\log^l{n})$ bit binary string. For each node $v$ in the skeleton, assign a variable $x_v$ using space $O(\log^l{n})$, to indicate the index of the gate that this node be labeled. This variable is also seen as a group of $O(\log^l{n})$ boolean variables. For each pair of connected nodes $u,v$ in the skeleton, and for each pair of possible indices $a,b$, which can be assigned to $x_u$ and $x_v$ correspondingly satisfying the conditions of a proof tree, create a clause encoding $x_u=a\wedge x_v=b$. All these clauses form an $\sat$ instance whose incidence graph has a tree decomposition with tree width $O(\log^l{n})$(See Figure~\ref{fig:logcfl_hard} for an example and illustration). This completes the proof.

\subsection{Proof of {Lemma}\ref{lem:search_cutting_depth}}
\begin{proof}
For any $h$, we can test whether $MCD_{c}(T, \emptyset)\leq h$ in
$O^{*}\left(n^{d}\right)$ using the following algorithm. The
algorithm is based on depth-first-search. For any tree $T$ and
previous cutting nodes $S$, to determine whether $MCD_{c}(T,
\emptyset)\leq h$, we can try all possible cutting node, then check
whether the minimal cutting depth of all subtrees is at most $h-1$
recursively. Since the depth of the search is at most $h$, so the
running time is $O^{*}\left(n^{h}\right)$. Therefore, the overall
time is at most $O^{*}\left(n^{MCD_{c}(T, \emptyset)}\right)$. The
space required is polynomial.
\end{proof}
